# Supplementary material for: The Use of Presence Data in Modelling Demand for Transportation
Source: arXiv:1802.03734 source file (2018-02-11)
Supplement: Supplementary file 1 [file additionalexperiments.tex]

\section{Additional Computational Experiments}
\label{adexperiments}

To corroborate the bounds on the run-time presented in Theorems~\ref{thm:tracemax},
we present a results on a benchmark suggested by Cuturi \cite{Cuturi2013}. 
Specifically, we compare the methods of 
Rubner et al. \cite{RubnerTomasiGuibas2000},
Cuturi \cite{Cuturi2013},
Pele and Werman \cite{5459199}, referenced above, 
with our algorithm of Theorem~\ref{thm:tracemax}.
Notice that 
the implementation of ours and of \cite{Cuturi2013} are in Matlab, while 
the implementation of \cite{RubnerTomasiGuibas2000} and \cite{5459199}
are in C linked via MEX interfaces (\texttt{emd\_mex}, \texttt{emd\_hat\_gd\_metric}).
Also, the implementation of \cite{RubnerTomasiGuibas2000} is limited to $n=512$ or less, in practice.
As in \cite{Cuturi2013}, vectors in the $n$-dimensional simplex are generated 
for an increasing $n$.
The mean and standard deviations of the run-time for each method are plotted in Figure~\ref{fig:comptime}
as a function of dimension $n$. The asymptotes are clear.

\begin{figure}\centering
\centering
\includegraphics[width=.5\textwidth]{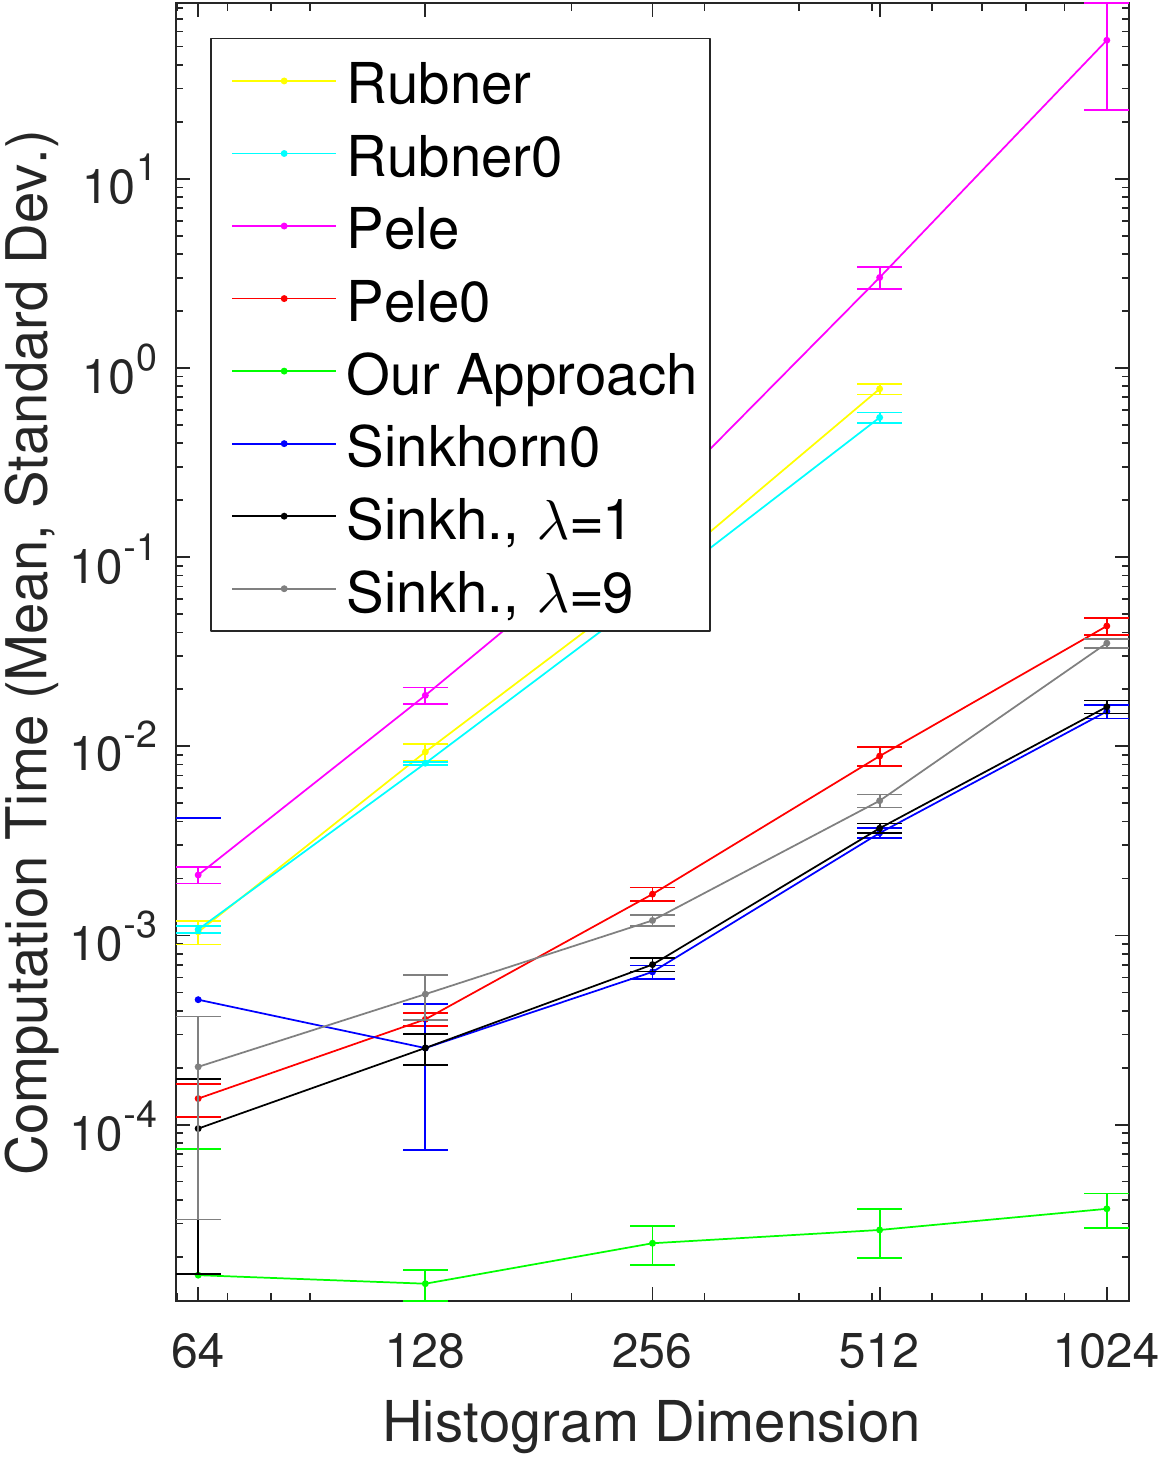}
\caption{Run-time of EMD computations as a function of dimension $n$, with vectors sampled from the $n$-dimensional simplex
and mean and standard deviation displayed.}\label{fig:comptime}
\end{figure}
